# Supplementary material for: Complexity-aware Large Scale Origin-Destination Network Generation via Diffusion Model
Source: arXiv:2306.04873 source file (2023-06-09)
Supplement: Supplementary file 1 [file Secend_appendix.tex]

\begin{figure*}[t]
    \centering
    \includegraphics[width=0.90\textwidth]{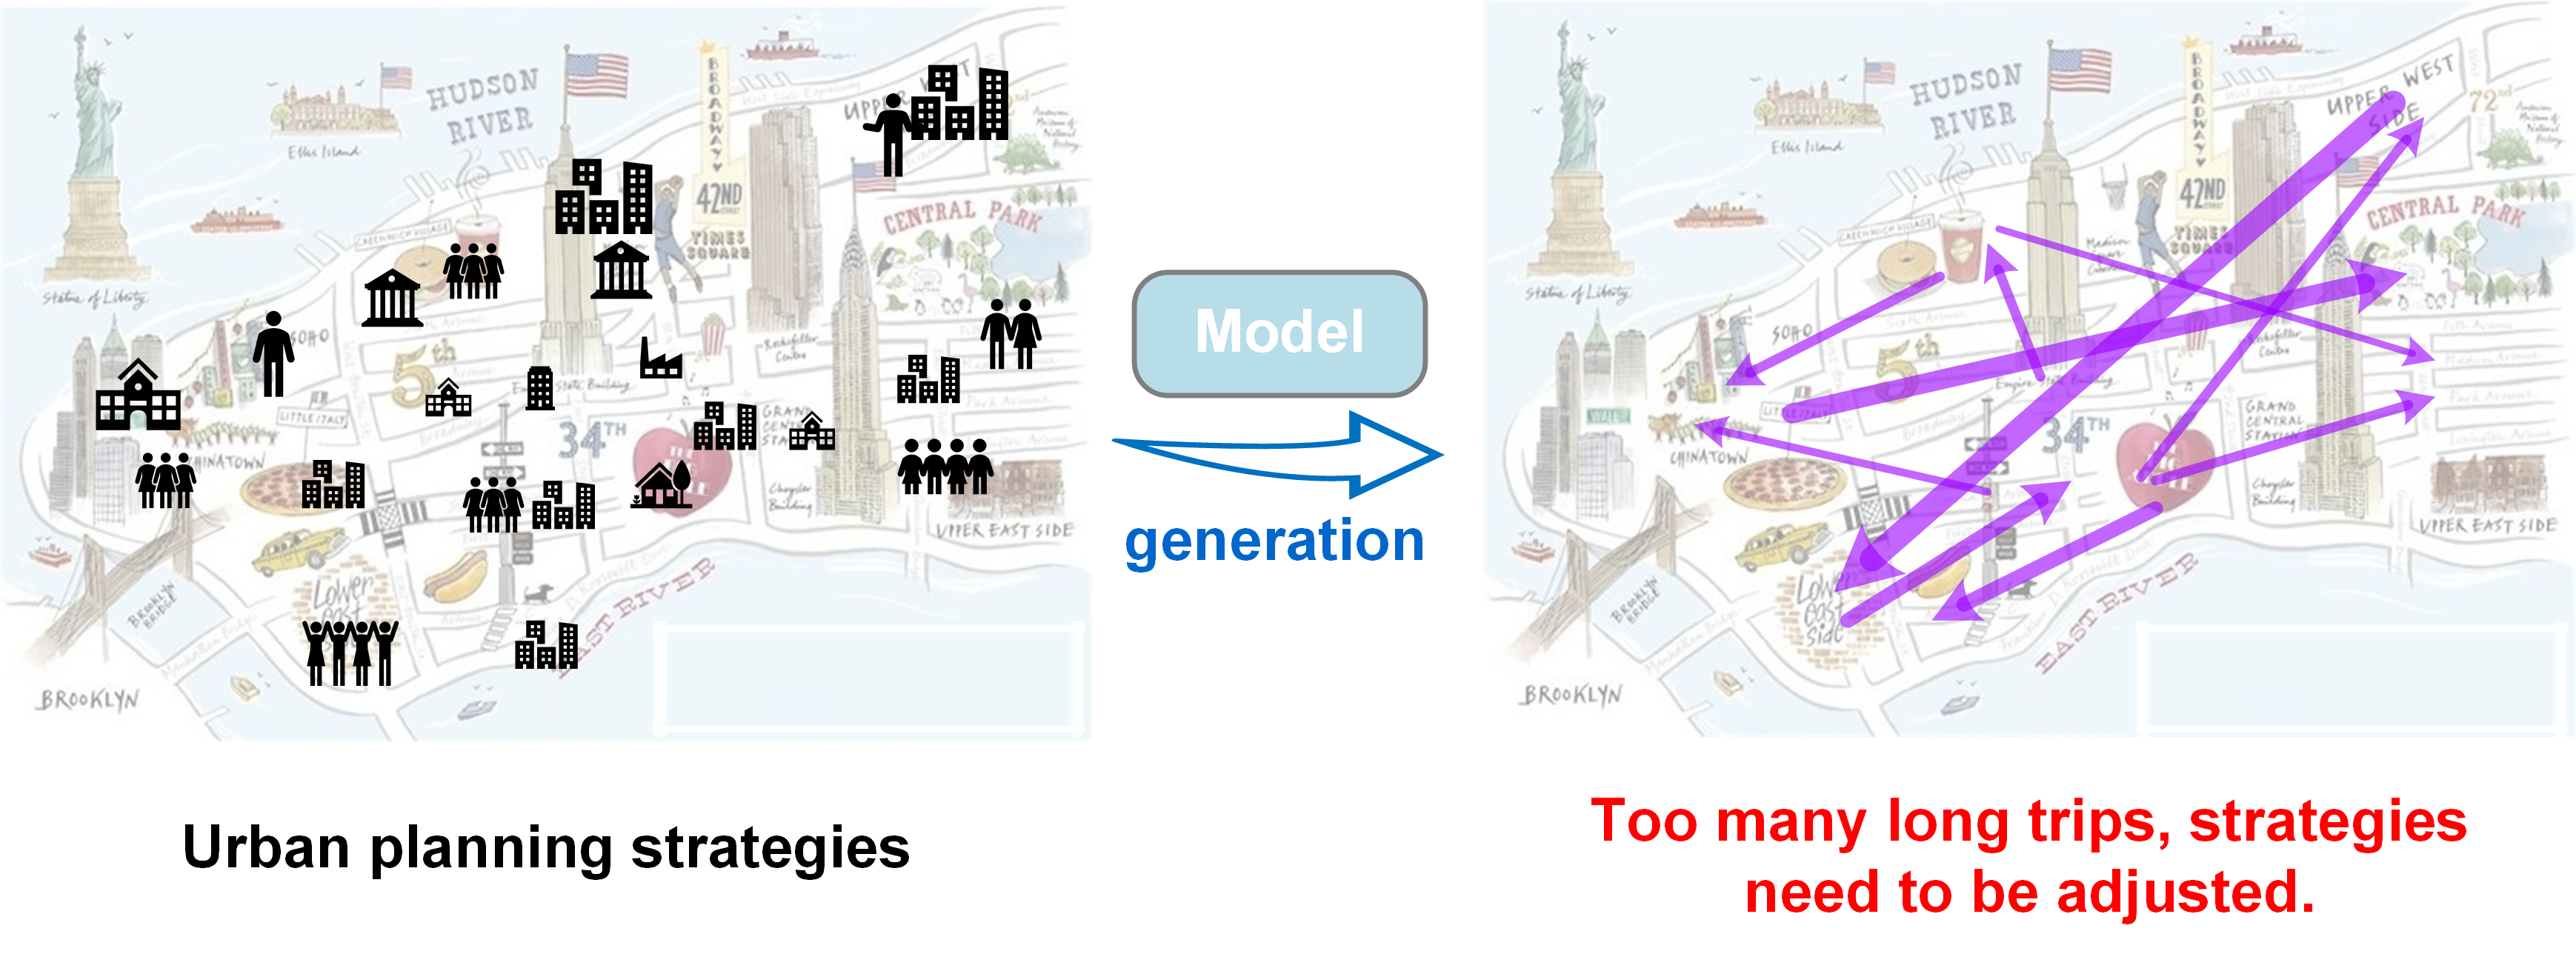}
    \caption{The illustration of the city-wide OD matrix generation problem and its practical applications.}
    \label{fig:illu}
\end{figure*}
